# Supplementary material for: Label, Verify, Correct: A Simple Few Shot Object Detection Method
Source: arXiv:2112.05749 source file (2022-03-29)
Supplement: Supplementary file 1 [file 00a-plan.tex]

% !TEX root = ../supplementary_material.tex
\section{Plan}

\subsection{Mentioned in the Paper}
\subsubsection{Limitations}
\begin{itemize}
    \item Experiments for LVIS which is a larger vocabulary expansion
    \item Ignore regions - can we somehow enforce images to be fully labelled
    \item Multiple iterations of the method - noisy label learning/clustering instead
\end{itemize}
\subsubsection{Ethical Concerns}

\subsubsection{Supervision Collapse}
\paragraph{False Positives - Class confusion}
\paragraph{False Negatives - Poor recall}
\begin{itemize}
    \item First show the lack of RPN recall with base trained RPN
    \item Missed detections: TFA vs. Our Baseline vs. Ideal Faster R-CNN (same images)
\end{itemize}

\subsubsection{Ignore Regions}
\begin{itemize}
    \item Show images with:
    \begin{itemize}
        \item pseudo-annotations with all examples labelled (no need for ignore regions)
        \item pseudo-annotations with some examples missing (no ignore regions visible)
        \item pseudo-annotations with some exampels missing (ignore regions visible and their utility shown)
    \end{itemize}
    \item Ablation: Table w/ our model with and without ignore regions
\end{itemize}

% \begin{figure*}[!htb]
% \centering
% \scriptsize
% \includegraphics[width=\linewidth]{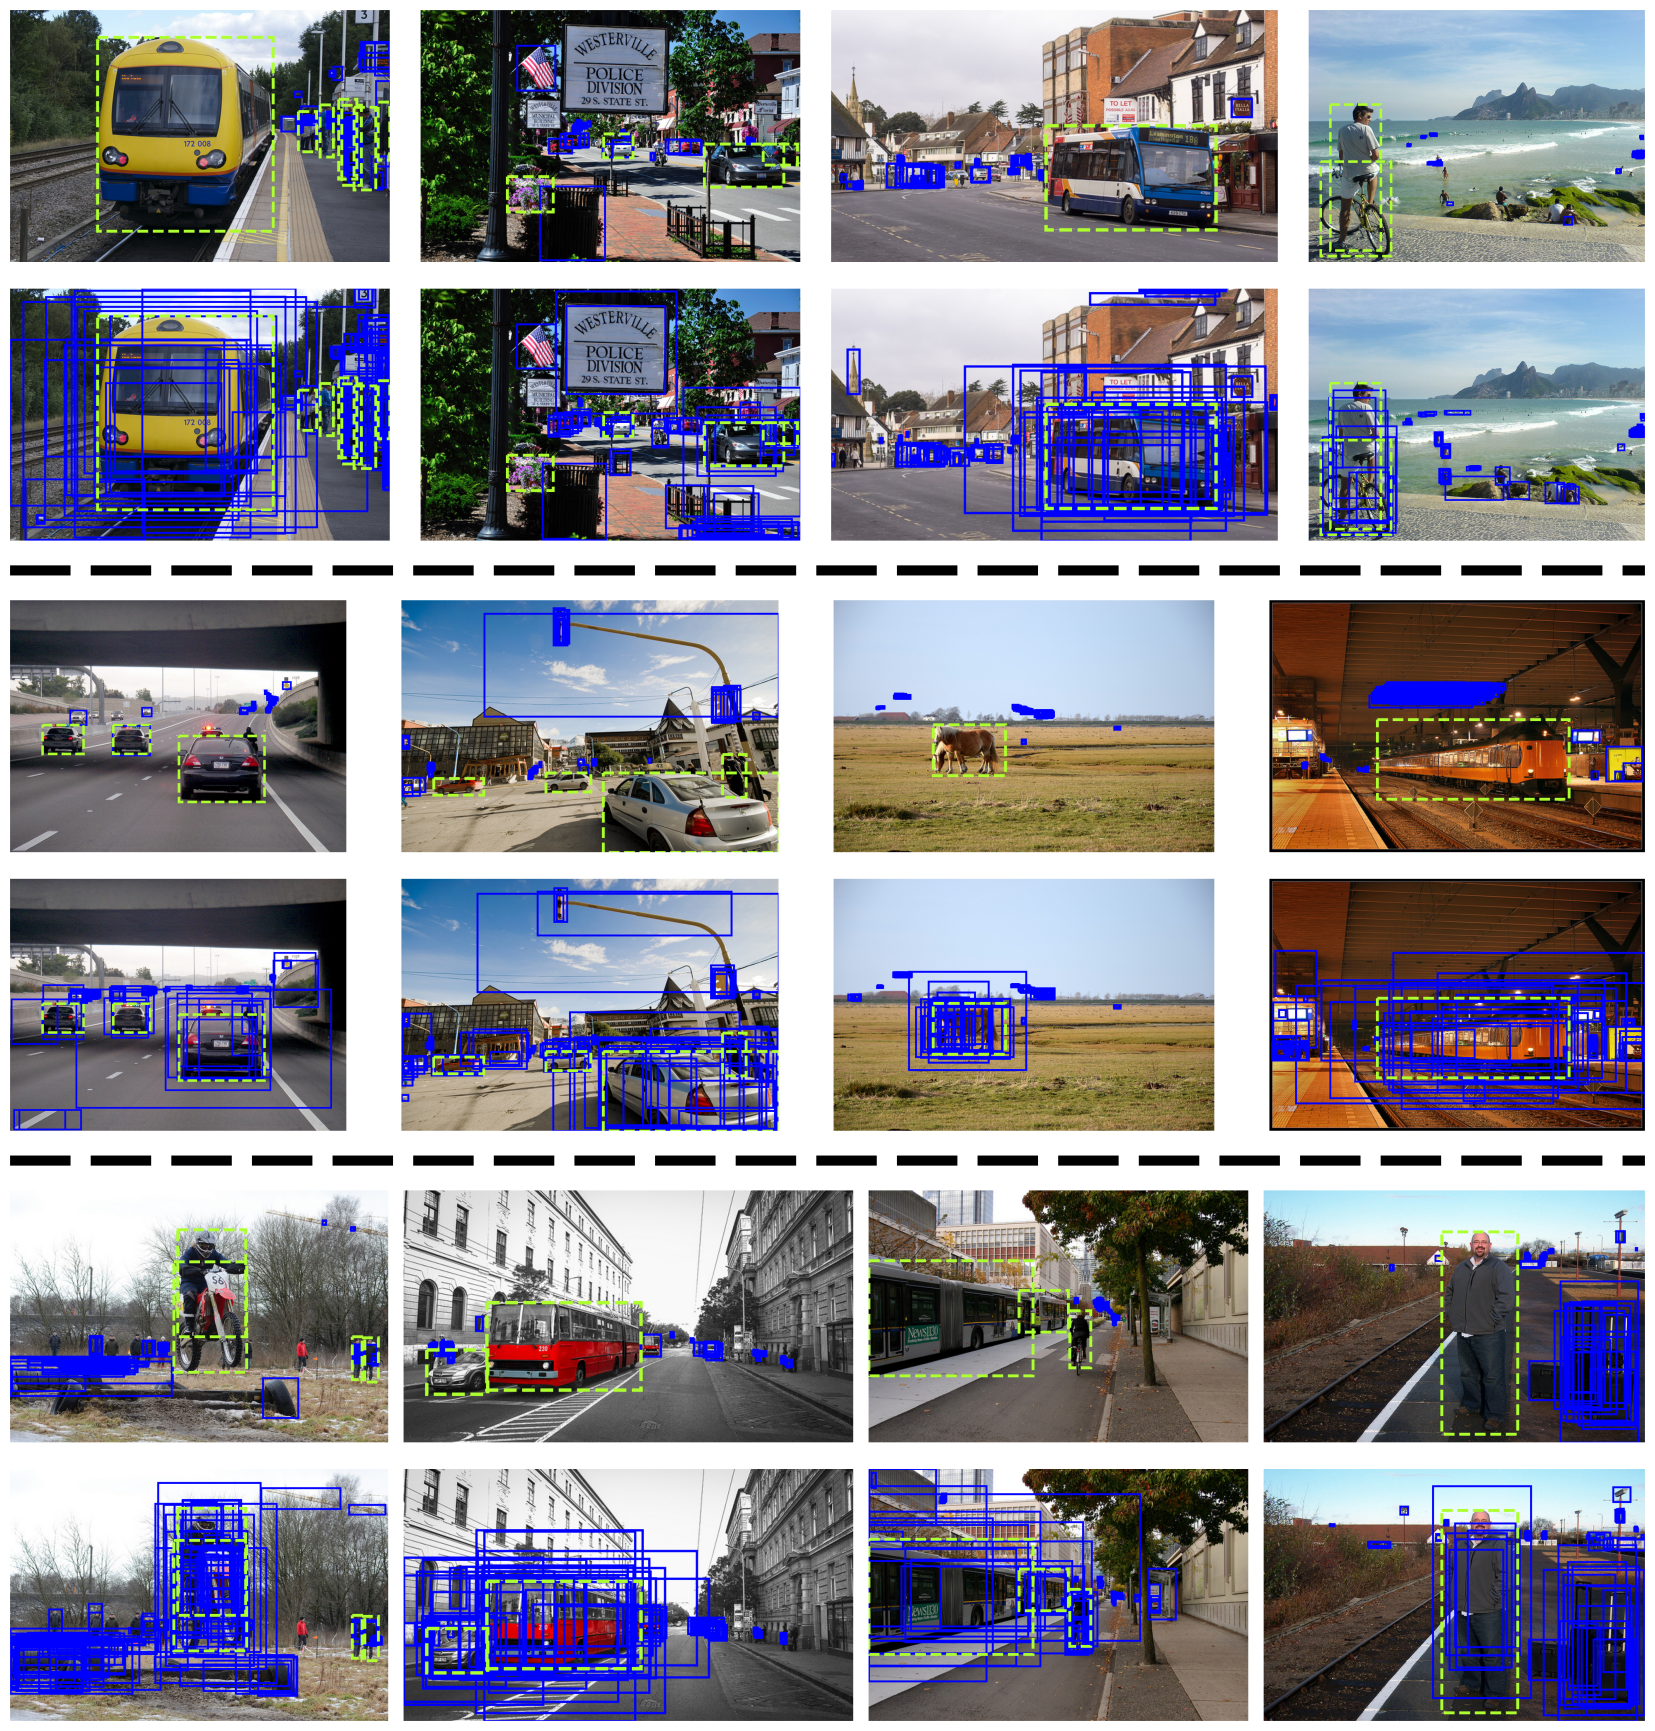}
% \vspace{-0.4cm}
% \caption{
% \hl{TODO} RPN trained only on Base vs RPN finetuned on novel data}
% % \caption{\hl{TO DO}}
% \label{fig:rpn_base_ft}
% \end{figure*}

% \begin{figure*}[!htb]
% \centering
% \scriptsize
% \includegraphics[width=\linewidth]{sm_assets/sm_images/fast_rcnn_supervision_collapse.pdf}
% \vspace{-0.4cm}
% \caption{
% \hl{TODO} TFA incorrectly puts positive RPN proposals into background, our modifications to training prevent this form of supervision collapse}
% % \caption{\hl{TO DO}}
% \label{fig:tfa_supervision_collapse}
% \end{figure*}

\subsubsection{}
