# Supplementary material for: Label, Verify, Correct: A Simple Few Shot Object Detection Method
Source: arXiv:2112.05749 source file (2022-03-29)
Supplement: Supplementary file 2 [file 00-sm-metadata.tex]

% !TEX root = ../supplementary_material.tex
\title{\textsc{Label, Verify, Correct: \\A Simple Few Shot Object Detection Method \\[5pt]
               (Supplementary Material)}}

\author{Prannay Kaul \qquad Weidi Xie \qquad Andrew Zisserman\\
Visual Geometry Group, University of Oxford\\
{\tt\small \{prannay, weidi, az\}@robots.ox.ac.uk}
% For a paper whose authors are all at the same institution,
% omit the following lines up until the closing ``}''.
% Additional authors and addresses can be added with ``\and'',
% just like the second author.
% To save space, use either the email address or home page, not both
% \and
% Second Author\\
% Institution2\\
% First line of institution2 address\\
% {\tt\small secondauthor@i2.org}
}
